# Supplementary material for: Accelerating equilibrium isotope effect calculations: II. Stochastic implementation of direct estimators
Source: arXiv:1909.02910 ancillary file (2019-10-26)
Supplement: Supplementary file 1 [file Karandashev_Vanicek_SDE_2019_SM.pdf]

# Supplementary material for "Accelerating equilibrium isotope effect calculations: II. Stochastic implementation of direct estimators"


Konstantin Karandashev[1, a)] and Jiří Vaníček[1, b)]

*Laboratory of Theoretical Physical Chemistry, Institut des Sciences et Ingénierie Chimiques, Ecole Polytechnique Fédérale de Lausanne (EPFL), CH-1015, Lausanne, Switzerland*



(Dated: August 19, 2019)


## I. DETERMINING SEVERAL ISOTOPE EFFECTS AT ONCE

A convenient feature of the direct estimator approach of Refs. 1 and 2 is the possibility to compute several isotope effects at once simply by averaging several direct estimators during one Monte Carlo or molecular dynamics simulation. Likewise, the thermodynamic integration and stepwise direct estimator approaches also allow computing at least the "intermediate" isotope effects as a by-product of one "overall" isotope-effect calculation: for example, to evaluate all isotope effects of the form $CH_{4-x}D_x/CH_4$ (x= $1, \dots, 4$) one can change inverse of the square root of the mass of the first hydrogen atom over the $\lambda$-interval $[0, 1/4]$, of the second atom over $\lambda \in [1/4, 2/4]$, etc. In this Supplementary Information we test numerical performance of TI, DE, SDE, and STI used with such a "sequential" procedure for changing mass and compare it to ODE results from Subsections III C and III D.

### A. Numerical details

The number of Monte Carlo steps, number of estimator evaluations, etc. of TI, DE, SDE, and STI calculations presented in this Supplementary Information are largely the same as the one from Subsections III C and III D. The main difference is that the mass interpolation procedure makes hydrogen atoms no longer equal, necessitating a way to shuffle the order in which their masses are changed during the calculation to decrease statistical error. The simplest way to achieve this is with simple $\lambda$-moves [Eqs. (19)-(23) of Ref. 3] with the trial moves part [Eqs. (19)-(22) of Ref. 3] modified to shuffle order of mass change without changing $\lambda$,[4] which can be added to a simulation with a negligible additional cost; $2 \times 10^8$ of these moves were added to all TI, DE, SDE, and STI calculations. For mass-scaled $\lambda$-moves in STI and SDE calculations, we modified the trial $\lambda$-move to attempt simultaneously changing $\lambda$ and shuffling the order in which hydrogen masses are changed. For the DE and TI simulations, we also checked how statistical error is affected by replacing 10% of Monte Carlo steps with respect to $\mathbf{r}$ with mass-scaled $\lambda$-moves that only attempt to shuffle the mass change order.

### B. Methane deuteration

We evaluate the $CD_4/CH_4$ isotope effect as in Subsec. III C except that atom masses are now changed according to the procedure described in the beginning of this section, which permits us to evaluate simultaneously and efficiently all isotope effects of the form $CH_{4-x}D_x/CH_4$ ($x = 1, \dots, 3$) as by-products. The resulting $CD_4/CH_4$ isotope effects are plotted in Fig. 1 with the ODE results from Subsec. III C added for comparison. As expected, the isotope effects evaluated with different methods agree [panel (a)], although TI exhibits a significant integration error in the high temperature limit [panel (b)]. The root mean square errors are plotted in panel (c); it is clear that changing hydrogen masses one by one increases statistical errors associated with TI and DE to the point that they are larger than the statistical error of ODE, especially for lower temperatures. Adding mass-scaled "shuffling" $\lambda$-moves or incorporating the stochastic change of mass (i.e. using STI or SDE) corrects this problem to a large extent, but the resulting methods still exhibit larger statistical errors compared to ODE over a wide range of temperatures. For future reference, the $CD_4/CH_4$ isotope effects obtained with all methods are presented in Table I, while the $CH_{4-x}D_x/CH_4$ isotope effects obtained with SDE are presented in Table II. The path integral discretization errors are not shown because they are the same as in the corresponding tables in the main text.

### C. Methanium deuteration

The $CD_5^+/CH_5^+$ isotope effect calculations were carried out analogously to those of $CD_4/CH_4$ discussed in the previous subsection, with isotope effects of the form $CH_{5-x}D_x^+/CH_5^+$ ($x = 1, \dots, 4$) evaluated as byproducts. The resulting $CD_5^+/CH_5^+$ isotope effects are plotted in Figure 2 with the ODE results from Subsec. III C added for comparison. The tendencies observed in the isotope effect values [panel (a)], integration errors [panel (b)], and statistical errors [panel (c)] are largely the same as those for methane, already discussed in the previous subsection, except that DE and TI without mass-scaled $\lambda$-moves exhibit even worse statistical errors compared to other


a) Electronic mail: konstantin.karandashev@alumni.epfl.ch
b) Electronic mail: jiri.vanicek@epfl.ch

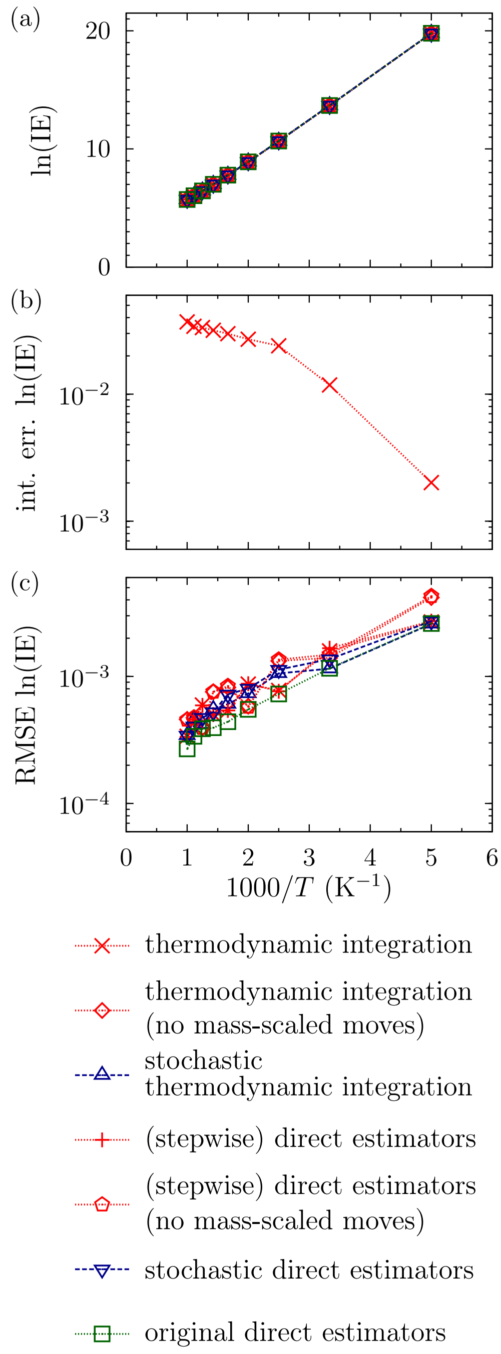


Figure 1. Calculations of the $CD_4/CH_4$ isotope effect (IE) obtained while hydrogen masses are changed one by one (see Subsec. I B). The three panels show the temperature dependence of (a) the isotope effect, (b) its integration errors, and (c) its statistical root mean square errors (RMSEs). For integration errors stochastic direct estimators values were used as the reference.

methods (compared with Figure 1). For future reference, the $CD_5^+/CH_5^+$ isotope effects obtained with all methods are presented in Table III, while the $CH_{5-x}D_x{}^+/CH_5^+$ isotope effects obtained with SDE are presented in Table IV. The path integral discretization errors are not shown because they are the same as in the corresponding tables in the main text.

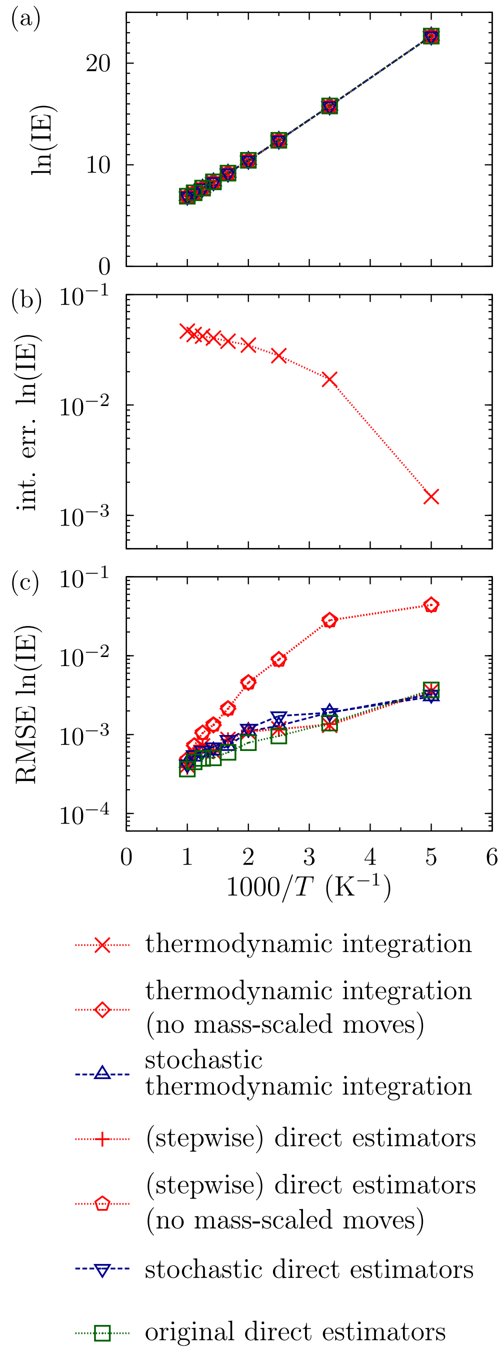


Figure 2. Root mean square errors of the $CD_5^+/CH_5^+$ isotope effect (IE) obtained with hydrogen masses changed one by one (see Subsec. I C).

Interestingly, the isotope effects at lower values of x are quite similar to the corresponding isotope effects calculated for deuteration of methane in Table II. A possible explanation is related to our discussion in Subsec. III D of the main text and follows from two qualitative tendencies: the main contributions to an isotope effect should

come from the most rigid internal degrees of freedom, as can be qualitatively seen from the harmonic approximation to the isotope effect,[5,6] and the most rigid degrees of freedom of methanium and its deuterated isotopologues correspond[7–9] to movements inside the $CH_3$ moiety which is structurally similar to the one inside methane.

## II. CONVERGENCE OF SHORTER CALCULATIONS FOR THE HARMONIC OSCILLATOR

In Subsec. III C of the main text we mentioned how STI and SDE are more suited for short calculations of isotope effects then TI and DE when exploration of $\lambda$ dimension with the Monte Carlo procedure is much faster than exploration of $\mathbf{r}$, which seems to be the case in most realistic systems. Harmonic oscillator is a model system where this is not the case because $\mathbf{r}$ can be sampled analytically by transforming to mass-scaled normal modes. In this section we demonstrate this by running calculations for the harmonic model with $\beta\hbar\omega_0 = 32$ that are completely analogous to those done for methane in Subsec. III C and plotted in Figure 3 of the main text, the only difference being that $J = 8$ is used for mass discretization. The results are plotted in Fig. 3. Direct sampling allows TI and DE values to converge almost instantaneously, while STI (and, to a much smaller extent, SDE) take time to converge as they involve sampling with respect to $\lambda$ which is not analytic. However, convergence of both SDE and STI is extremely quick in this case, indicating effectiveness of our Monte Carlo procedure for sampling $\lambda$, at least for harmonic systems; in fact it seems faster than convergence of ODE.

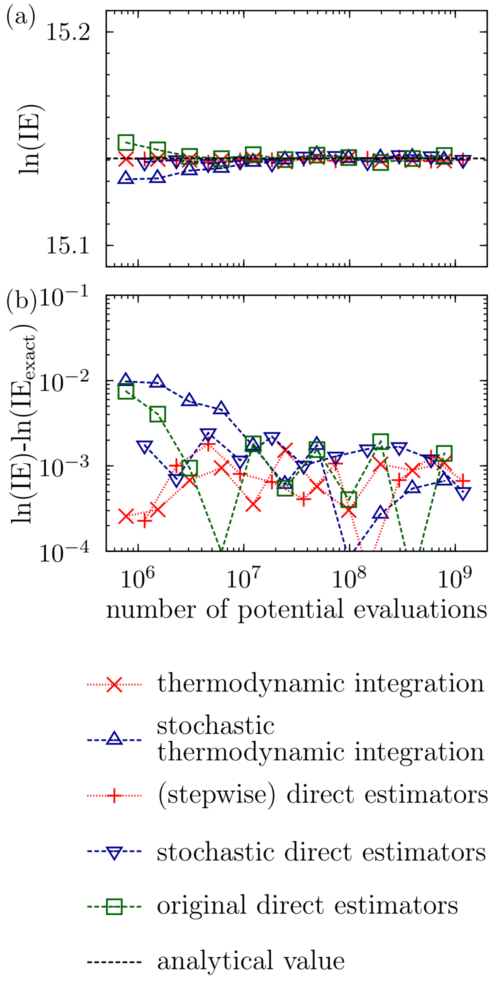


Figure 3. The impact of nonergodicity appearing in shorter calculations of the isotope effect in the harmonic model used in Ref. 3. Panel (a) presents the convergence of the IE as a function of the simulation length, while panel (b) shows the corresponding error of the IE (in logarithmic scale) relative to the analytic result.

## REFERENCES


[1] A. Pérez and O. A. von Lilienfeld, J. Chem. Theory Comput. **7**, 2358 (2011).

[2] B. Cheng and M. Ceriotti, J. Chem. Phys. **141**, 244112 (2015).

[3] K. Karandashev and J. Vaníček, J. Chem. Phys. **146**, 184102 (2017).

[4] J. Liu, R. S. Andino, C. M. Miller, X. Chen, D. M. Wilkins, M. Ceriotti, and D. E. Manolopoulos, J. Phys. Chem. C **117**, 2944 (2013).

[5] H. C. Urey, J. Chem. Soc. **1947**, 562 (1947).

[6] M. Wolfsberg, W. A. V. Hook, P. Paneth, and L. P. N. Rebelo, *Isotope Effects in the Chemical, Geological and Bio Sciences* (McGraw-Hill, 2010).

[7] X. Huang, A. B. McCoy, J. M. Bowman, L. M. Johnson, C. Savage, F. Dong, and D. J. Nesbitt, Science **311**, 60 (2006).

[8] S. D. Ivanov, O. Asvany, A. Witt, E. Hugo, G. Mathias, B. Redlich, D. Marx, and S. Schlemmer, Nat. Chem. **2**, 298 (2010).

[9] S. D. Ivanov, A. Witt, and D. Marx, Phys. Chem. Chem. Phys. **15**, 10270 (2013).

Table I. Values of the $CD_4/CH_4$ isotope effect (IE) obtained with thermodynamic integration (TI), stochastic thermodynamic integration (STI), direct estimators (DE), and "stochastic direct estimators" (SDE). Statistical errors are root mean square errors estimated with block averaging. Mass was changed one hydrogen at a time as explained in the beginning of this section. The proposed methodology is SDE.

| $T$(K) | TI: mass-scaled moves added, yes | TI: mass-scaled moves added, no | DE: mass-scaled moves added, yes | DE: mass-scaled moves added, no | STI | SDE |
|---|---|---|---|---|---|---|
| 200 | $19.786 \pm 0.003$ | $19.780 \pm 0.005$ | $19.789 \pm 0.003$ | $19.781 \pm 0.005$ | $19.789 \pm 0.003$ | $19.784 \pm 0.003$ |
| 300 | $13.660 \pm 0.002$ | $13.658 \pm 0.002$ | $13.675 \pm 0.002$ | $13.673 \pm 0.002$ | $13.673 \pm 0.002$ | $13.672 \pm 0.002$ |
| 400 | $10.644 \pm 0.001$ | $10.642 \pm 0.002$ | $10.666 \pm 0.001$ | $10.664 \pm 0.002$ | $10.665 \pm 0.002$ | $10.668 \pm 0.002$ |
| 500 | $8.882 \pm 0.001$ | $8.884 \pm 0.001$ | $8.909 \pm 0.001$ | $8.910 \pm 0.001$ | $8.910 \pm 0.001$ | $8.909 \pm 0.001$ |
| 600 | $7.750 \pm 0.001$ | $7.750 \pm 0.001$ | $7.780 \pm 0.001$ | $7.779 \pm 0.001$ | $7.780 \pm 0.001$ | $7.780 \pm 0.001$ |
| 700 | $6.974 \pm 0.001$ | $6.975 \pm 0.001$ | $7.006 \pm 0.001$ | $7.007 \pm 0.001$ | $7.006 \pm 0.001$ | $7.006 \pm 0.001$ |
| 800 | $6.417 \pm 0.001$ | $6.417 \pm 0.001$ | $6.451 \pm 0.001$ | $6.451 \pm 0.001$ | $6.451 \pm 0.001$ | $6.450 \pm 0.001$ |
| 900 | $6.004 \pm 0.001$ | $6.003 \pm 0.001$ | $6.039 \pm 0.001$ | $6.039 \pm 0.001$ | $6.040 \pm 0.001$ | $6.038 \pm 0.001$ |
| 1000 | $5.688 \pm 0.001$ | $5.689 \pm 0.001$ | $5.725 \pm 0.001$ | $5.726 \pm 0.001$ | $5.726 \pm 0.001$ | $5.726 \pm 0.001$ |

Table II. Temperature dependence of the $CH_{4-x}D_x/CH_4$ isotope effect for x = 1, 2, 3. The results were obtained with stochastic direct estimators, the statistical errors are root mean square errors estimated with block averaging.

| $T$(K) | ln(IE) ($CH_{4-x}D_x/CH_4$): x=1 | x=2 | x=3 |
|---|---|---|---|
| 200 | $4.874 \pm 0.002$ | $9.802 \pm 0.002$ | $14.769 \pm 0.003$ |
| 300 | $3.386 \pm 0.001$ | $6.794 \pm 0.001$ | $10.223 \pm 0.002$ |
| 400 | $2.652 \pm 0.001$ | $5.314 \pm 0.001$ | $7.985 \pm 0.001$ |
| 500 | $2.218 \pm 0.001$ | $4.443 \pm 0.001$ | $6.673 \pm 0.001$ |
| 600 | $1.940 \pm 0.001$ | $3.883 \pm 0.001$ | $5.830 \pm 0.001$ |
| 700 | $1.748 \pm 0.001$ | $3.499 \pm 0.001$ | $5.251 \pm 0.001$ |
| 800 | $1.610 \pm 0.001$ | $3.222 \pm 0.001$ | $4.835 \pm 0.001$ |
| 900 | $1.508 \pm 0.001$ | $3.017 \pm 0.001$ | $4.527 \pm 0.001$ |
| 1000 | $1.430 \pm 0.001$ | $2.861 \pm 0.001$ | $4.293 \pm 0.001$ |

Table III. Values of the $CD_5^+/CH_5^+$ isotope effect (IE) obtained with thermodynamic integration (TI), stochastic thermodynamic integration (STI), direct estimators (DE), and "stochastic direct estimators" (SDE). Statistical errors are root mean square errors estimated with block averaging. Mass was changed one hydrogen at a time as explained in the beginning of this section. The proposed methodology is SDE.

| $T$(K) | TI: mass-scaled moves added, yes | TI: mass-scaled moves added, no | DE: mass-scaled moves added, yes | DE: mass-scaled moves added, no | STI | SDE |
|---|---|---|---|---|---|---|
| 200 | $22.675 \pm 0.004$ | $22.69 \pm 0.05$ | $22.670 \pm 0.004$ | $22.69 \pm 0.05$ | $22.673 \pm 0.004$ | $22.673 \pm 0.004$ |
| 300 | $15.772 \pm 0.002$ | $15.76 \pm 0.03$ | $15.788 \pm 0.002$ | $15.78 \pm 0.03$ | $15.785 \pm 0.002$ | $15.789 \pm 0.002$ |
| 400 | $12.386 \pm 0.002$ | $12.387 \pm 0.009$ | $12.414 \pm 0.002$ | $12.414 \pm 0.009$ | $12.411 \pm 0.002$ | $12.414 \pm 0.002$ |
| 500 | $10.411 \pm 0.002$ | $10.422 \pm 0.005$ | $10.444 \pm 0.002$ | $10.456 \pm 0.005$ | $10.445 \pm 0.002$ | $10.445 \pm 0.002$ |
| 600 | $9.145 \pm 0.001$ | $9.144 \pm 0.003$ | $9.183 \pm 0.001$ | $9.181 \pm 0.003$ | $9.183 \pm 0.001$ | $9.183 \pm 0.001$ |
| 700 | $8.230 \pm 0.001$ | $8.278 \pm 0.002$ | $8.321 \pm 0.001$ | $8.319 \pm 0.002$ | $8.320 \pm 0.001$ | $8.320 \pm 0.001$ |
| 800 | $7.662 \pm 0.001$ | $7.662 \pm 0.002$ | $7.705 \pm 0.001$ | $7.705 \pm 0.002$ | $7.705 \pm 0.001$ | $7.704 \pm 0.001$ |
| 900 | $7.206 \pm 0.001$ | $7.205 \pm 0.001$ | $7.251 \pm 0.001$ | $7.250 \pm 0.001$ | $7.250 \pm 0.001$ | $7.249 \pm 0.001$ |
| 1000 | $6.857 \pm 0.001$ | $6.858 \pm 0.001$ | $6.904 \pm 0.001$ | $6.904 \pm 0.001$ | $6.905 \pm 0.001$ | $6.904 \pm 0.001$ |

Table IV. Temperature dependence of the $CH_{5-x}D_x^+/CH_5^+$ isotope effect for x = 1, . . . , 4; the results were obtained with stochastic direct estimators while changing hydrogen masses one by one.

| $T$(K) | ln(IE) ($CH_{5-x}D_x^+/CH_5^+$) | | | |
|---|---|---|---|---|
| | x=1 | x=2 | x=3 | x=4 |
| 200 | $4.547 \pm 0.002$ | $9.094 \pm 0.003$ | $13.629 \pm 0.003$ | $18.153 \pm 0.004$ |
| 300 | $3.159 \pm 0.001$ | $6.318 \pm 0.001$ | $9.475 \pm 0.002$ | $12.630 \pm 0.002$ |
| 400 | $2.482 \pm 0.001$ | $4.964 \pm 0.001$ | $7.446 \pm 0.002$ | $9.929 \pm 0.002$ |
| 500 | $2.088 \pm 0.001$ | $4.177 \pm 0.001$ | $6.266 \pm 0.001$ | $8.355 \pm 0.001$ |
| 600 | $1.836 \pm 0.001$ | $3.672 \pm 0.001$ | $5.509 \pm 0.001$ | $7.345 \pm 0.001$ |
| 700 | $1.663 \pm 0.001$ | $3.328 \pm 0.001$ | $4.992 \pm 0.001$ | $6.656 \pm 0.001$ |
| 800 | $1.541 \pm 0.001$ | $3.081 \pm 0.001$ | $4.622 \pm 0.001$ | $6.163 \pm 0.001$ |
| 900 | $1.449 \pm 0.001$ | $2.899 \pm 0.001$ | $4.349 \pm 0.001$ | $5.799 \pm 0.001$ |
| 1000 | $1.380 \pm 0.001$ | $2.761 \pm 0.001$ | $4.142 \pm 0.001$ | $5.523 \pm 0.001$ |
